# Supplementary material for: Incommensurate magnetic order drives singular angular magnetoresistance in a Weyl semimetal
Source: arXiv:2509.18398 source file (2025-09-22)
Supplement: Supplementary file 1 [file SM_PRL_5Sep25.pdf]

# Supplemental Material: Incommensurate magnetic order drives singular angular magnetoresistance in a Weyl semimetal

X. Yao,<sup>1</sup> P. Chen,<sup>2</sup> R. Verma,<sup>3</sup> X. Zhao,<sup>1</sup> H.-Y. Yang,<sup>1,4</sup> L. DeBeer-Schmitt,<sup>5</sup>  
A. A. Aczel,<sup>5</sup> C.-M. Wu,<sup>6</sup> D. Alba Venero,<sup>7</sup> T. Ohhara,<sup>8</sup> K. Munakata,<sup>9</sup> M. Takahashi,<sup>9</sup>  
Y. Noda,<sup>10,11</sup> A. Bansil,<sup>12,13</sup> B. Singh,<sup>3</sup> P. Nikolić,<sup>14,15</sup> F. Tafti,<sup>1</sup> and J. Gaudet<sup>2,16</sup>

<sup>1</sup>*Department of Physics, Boston College, Chestnut Hill, MA 02467, USA*

<sup>2</sup>*NIST Center for Neutron Research, National Institute of Standards and Technology, Gaithersburg, Maryland 20899, USA*

<sup>3</sup>*Department of Condensed Matter Physics and Materials Science,  
Tata Institute of Fundamental Research, Colaba, Mumbai 400005, India*

<sup>4</sup>*Department of Electrical and Computer Engineering,  
University of California, Los Angeles, CA, USA.*

<sup>5</sup>*Neutron Scattering Division, Oak Ridge National Laboratory, Oak Ridge, Tennessee 37831, USA*

<sup>6</sup>*National Synchrotron Radiation Research Center, Hsinchu 300092, Taiwan*

<sup>7</sup>*ISIS neutron and muon source, STFC, Rutherford Appleton Laboratory, Didcot, OX11 0QX, UK*

<sup>8</sup>*J-PARC Center, Japan Atomic Energy Agency, 2-4 Shirakata, Tokai, Ibaraki 319-1195, Japan*

<sup>9</sup>*Department of Materials Science, Institute of Pure and Applied Sciences,  
University of Tsukuba, Tsukuba, Ibaraki 305-8573, Japan*

<sup>10</sup>*Institute for Solid State Physics, The University of Tokyo, Kashiwa, Chiba 277-0882, Japan*

<sup>11</sup>*Institute of Multidisciplinary Research for Advanced Materials, Tohoku University, Sendai 980-8577, Japan*

<sup>12</sup>*Department of Physics, Northeastern University, Boston, Massachusetts 02115, USA*

<sup>13</sup>*Quantum Materials and Sensing Institute, Northeastern University, Burlington, Massachusetts 01803, USA*

<sup>14</sup>*Institute for Quantum Matter and William H. Miller III Department of Physics and Astronomy,  
Johns Hopkins University, Baltimore, Maryland 21218, USA*

<sup>15</sup>*Department of Physics and Astronomy, George Mason University, Fairfax, VA 22030, USA*

<sup>16</sup>*Department of Materials Science and Eng., University of Maryland, College Park, MD 20742-2115  
(Dated: September 21, 2025)*

## METHODS

Elemental compositions were confirmed using energy-dispersive X-ray spectroscopy (EDX) performed with a scanning electron microscope (SEM). Structural characterizations were conducted via powder X-ray diffraction (XRD). Heat capacity, electrical resistivity, and AC susceptibility measurements were performed using a Quantum Design Physical Property Measurement System (PPMS) with the DynaCool platform. DC magnetization was measured using a Magnetic Property Measurement System (MPMS).

We performed single-crystal neutron diffraction using the HB-1A thermal triple-axis spectrometer at ORNL ( $\lambda = 2.37$  Å) to probe CeAlGe and CeAlSi<sub>0.67</sub>Ge<sub>0.23</sub>, the 4-circle diffractometer FONDER ( $\lambda = 1.2464$  Å) at JRR-3 to probe CeAlSi and CeAlGe, and the time-of-flight diffractometer SENJU at J-PARC to probe CeAlSi<sub>0.27</sub>Ge<sub>0.63</sub>. All experiments were performed with a base temperature ranging between 2 K to 4 K. The FONDER experiment was performed in zero-field, while the HB-1A and SENJU experiments were conducted with a vertical field applied parallel to the **b**-axis of the crystal. In this case, the (H0L) reciprocal space of the crystal was lying within the horizontal plane of the spectrometers.

The SANS data shown in this work for CeAlSi was acquired with both the Zoom instrument at ISIS and the QUOKKA instrument at ANSTO. The data collected

on QUOKKA was obtained with a sample to detector distance of 20 m and an incident neutron wavelength of 8.1 Å (low-Q configuration). The ZOOM data was obtained with a sample to detector distance of 8 m using a polychromatic beam with neutrons from 1.75 Å to 15 Å. The GP-SANS instrument at HFIR in Oak Ridge National Laboratory was utilized to collect both the low-Q and high-Q SANS data for CeAlGe as well as CeAlSi<sub>0.27</sub>Ge<sub>0.63</sub> presented in this work. The low-Q (high-Q) configuration of our GP-SANS experiment corresponds to a sample to detector distance of 19 m (5 m) and an incident neutron wavelength of 12 Å (6 Å). For all SANS experiments, a flat-plate sample was mounted in a low-temperature cryostat (~2 K-3 K) with the **c**-axis parallel to the neutron beam so we could access the in-plane scattering vectors with the 2D SANS detector. A [110] field was used for the ANSTO experiment, while a [010] field was used for the GP-SANS experiment. All the SANS data were collected for rocking angles typically varying from  $\pm 6^\circ$ . A high-field or high-temperature background measurement was also subtracted from the data. Error bars associated with all neutron diffraction intensities reported in this work correspond to 1 standard deviation.

## CRYSTAL GROWTH AND STRUCTURE

All CeAlSi<sub>1-x</sub>Ge<sub>x</sub> single crystals were grown using a self-flux method [1] in standard alumina crucibles.

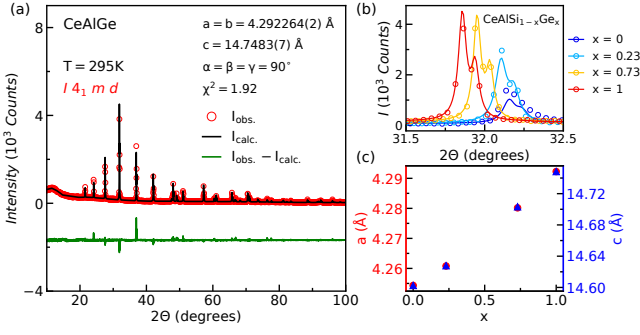

FIG. S1. X-ray refinement for (a) CeAlSi, (b) for CeAlSi<sub>1-x</sub>Ge<sub>x</sub> highlighting the main peak region; (c) Lattice parameter  $a$  and  $c$  as a function of the doping level  $x$ .

The starting materials were weighed in a molar ratio of Ce:Al:(Si+Ge) = 1:10:1, loaded into a crucible sealed in an evacuated quartz tube, and heated to 1000 °C at a rate of 3°C/min. The mixture was held at 1000 °C for 12 hours, then slowly cooled to 700 °C at a rate of 0.1 °C/min, held at that temperature for another 12 hours, and finally centrifuged to remove residual Al flux.

The structures of the single crystals were characterized using powder X-ray diffraction (XRD) and energy-dispersive X-ray spectroscopy (EDX). Second-harmonic generation (SHG) measurements, as reported in Ref. [1], were used to distinguish between the noncentrosymmetric I4<sub>1</sub>md (No.109) and centrosymmetric I4<sub>1</sub>/amd (No.141) space groups.

3-hour long-scan XRD measurements were performed with sample rotation to aid structural refinement and extract lattice parameters. The results are summarized in Fig. S1. For EDX measurements, the electron beam was operated at 20 keV with a beam current of 0.4 nA. Three different spots on each crystal were scanned to determine the average and standard deviation of the atomic percentages. The final compositions and their associated errors are summarized in Table I.

| Nomical composition                       | EDX result                                                                               |
|-------------------------------------------|------------------------------------------------------------------------------------------|
| CeAlSi                                    | Ce <sub>0.93(4)</sub> Al <sub>1.02(2)</sub> Si                                           |
| CeAlSi <sub>0.90</sub> Ge <sub>0.10</sub> | Ce <sub>0.95(3)</sub> Al <sub>1.06(5)</sub> Si <sub>0.90(3)</sub> Ge <sub>0.10(1)</sub>  |
| CeAlSi <sub>0.80</sub> Ge <sub>0.20</sub> | Ce <sub>0.87(8)</sub> Al <sub>1.11(8)</sub> Si <sub>0.77(1)</sub> Ge <sub>0.23(1)</sub>  |
| CeAlSi <sub>0.72</sub> Ge <sub>0.28</sub> | Ce <sub>0.94(8)</sub> Al <sub>1.16(7)</sub> Si <sub>0.67(3)</sub> Ge <sub>0.33(2)</sub>  |
| CeAlSi <sub>0.50</sub> Ge <sub>0.50</sub> | Ce <sub>0.92(1)</sub> Al <sub>1.09(6)</sub> Si <sub>0.49(1)</sub> Ge <sub>0.51(1)</sub>  |
| CeAlSi <sub>0.45</sub> Ge <sub>0.55</sub> | Ce <sub>0.93(2)</sub> Al <sub>1.10(4)</sub> Si <sub>0.42(3)</sub> Ge <sub>0.58(2)</sub>  |
| CeAlSi <sub>0.40</sub> Ge <sub>0.60</sub> | Ce <sub>0.94(2)</sub> Al <sub>1.12(4)</sub> Si <sub>0.37(1)</sub> Ge <sub>0.63(2)</sub>  |
| CeAlSi <sub>0.28</sub> Ge <sub>0.72</sub> | Ce <sub>0.93(1)</sub> Al <sub>1.10(7)</sub> Si <sub>0.27(1)</sub> Ge <sub>0.73(1)</sub>  |
| CeAlSi <sub>0.25</sub> Ge <sub>0.75</sub> | Ce <sub>0.92(1)</sub> Al <sub>1.08(7)</sub> Si <sub>0.25(1)</sub> Ge <sub>0.75(2)</sub>  |
| CeAlSi <sub>0.18</sub> Ge <sub>0.82</sub> | Ce <sub>0.95(1)</sub> Al <sub>1.13(11)</sub> Si <sub>0.15(1)</sub> Ge <sub>0.85(1)</sub> |
| CeAlSi <sub>0.02</sub> Ge <sub>0.98</sub> | Ce <sub>0.97(4)</sub> Al <sub>1.15(10)</sub> Si <sub>0.03(1)</sub> Ge <sub>0.97(2)</sub> |
| CeAlGe                                    | Ce <sub>0.96(3)</sub> Al <sub>1.07(5)</sub> Ge                                           |

TABLE I. EDX result tabulated for all CeAlSi<sub>1-x</sub>Ge<sub>x</sub> samples in this study.

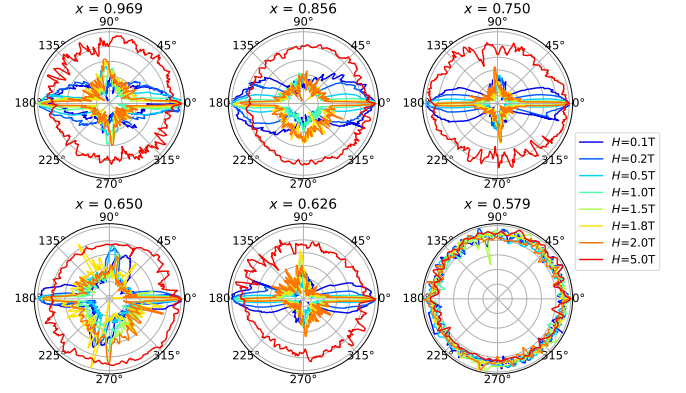

FIG. S2. Angular magneto-resistance for CeAlSi<sub>1-x</sub>Ge<sub>x</sub>. SAMR could be observed in  $x > 0.579$  and  $H < 3$  T.

## ANGULAR DEPENDENCE IN MAGNETO-RESISTANCE

Fig. S2 presents the normalized longitudinal resistivity  $\rho_{xx}$  as a function of the rotation angle in the  $ab$  plane for multiple compositions of CeAlSi<sub>1-x</sub>Ge<sub>x</sub> under different magnetic fields. The angular dependence is observed for all compositions when  $x > x_c$  ( $x_c \approx 0.58$ ); however, singular angular magnetoresistance (SAMR), the strikingly sharp and field-sensitive peaks, are only found for those compositions with field  $1 \text{ T} < H < 3 \text{ T}$ . Above this field, the signal begins to broaden and gradually deviates from the singular shape.

In contrast, samples with  $x < x_c$  exhibit more conventional AMR behavior with nearly no angular dependence at low fields. Fig. S3 provides a clearer view of the relationship between the singularity (defined as the inverse of the full width at half maximum of the peak) and magnetic field, as also shown in Fig.3(d) of the main text for comparison with the derivative of the neutron Bragg peak. We further combine these SAMR behavior with neutron diffraction, small-angle neutron scattering (SANS), and theoretical calculations to investigate the underlying mechanism, revealing a close connection to its complex spin magnetic ordering across the critical composition  $x_c$ .

## PHASE DIAGRAM

We combined heat capacity (Fig. S4(c)) and magnetism (Fig. S4(a), (b), (d), (e)) with SAMR to present the two phases shown in the main text Fig. 1(b), also in Fig. S4(f). AC susceptibility under low field ( $H = 100 \text{ Oe}$ ,  $H \parallel [110]$ ) shows sharp anomalies that track the antiferromagnetic transition temperature  $T_N$ , which is further corroborated by heat capacity and DC susceptibility data, highlighting a close correlation between magnetic ordering and the onset of SAMR above a critical composition. The phase transition temperature is summarized in Table II.

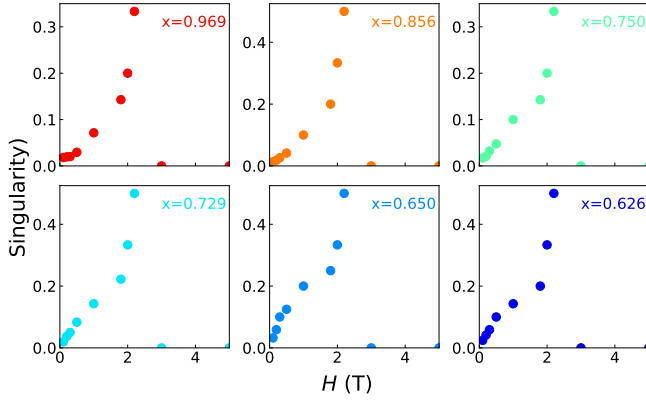

FIG. S3. Singularity derived from angular magneto-resistance for  $\text{CeAlSi}_{1-x}\text{Ge}_x$ .

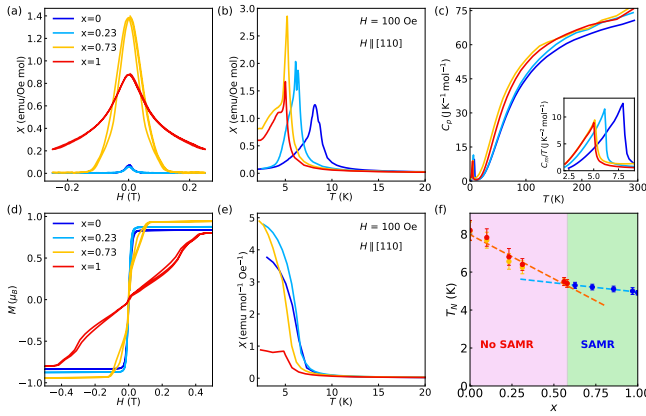

FIG. S4. AC susceptibility as a function of (a) field  $H$ , (b) temperature  $T$ , for  $\text{CeAlSi}_{1-x}\text{Ge}_x$ , with field  $H = 100\text{Oe}$ ,  $H \parallel [110]$ ; (c) Heat capacity at zero field; (d) DC magnetic moment  $M$  as a function of  $H$ ; (e) DC susceptibility as a function of  $T$ ; (f) phase diagram combining SAMR with transition temperature obtained from (b), (c), (e)

## SPIN STRUCTURE REFINEMENT

As described in the main text, all  $\text{CeAlSi}_{1-x}\text{Ge}_x$  crystals exhibit a single low-temperature magnetic phase transition at a critical temperature  $T_c$ , which ranges from approximately 5 K to 8 K depending on composition. Below  $T_c$ , all samples develop a commensurate magnetic order characterized by the propagation vector  $\mathbf{k} = \mathbf{0}$ . This is clearly illustrated in Fig. S5(a), which shows that the low-temperature Bragg intensity is increased below  $T_c$  for both structurally allowed reflections and symmetry-disallowed reflections at integer H, K, L positions, consistent with a  $\mathbf{k} = \mathbf{0}$  magnetic order. Single-crystal diffraction also clearly shows both incommensurate and commensurate peaks are present for  $x > x_c$  (Fig. S5(c,d)). The doping dependence of the temperature order parameter are shown in Fig. S5(b) and shows these peaks correlate with  $T_c$ .

Symmetry analysis identifies three irreducible represen-

| $x$     | $T_N$ from HC (K) | $T_N$ from magnetism (K) |
|---------|-------------------|--------------------------|
| 0       | 8.2(5)            | 8.2(5)                   |
| 0.10(1) | 7.7(4)            | 7.8(5)                   |
| 0.23(1) | 6.6(4)            | 6.8(4)                   |
| 0.33(2) | 6.3(3)            | 6.4(3)                   |
| 0.51(1) | 5.5(2)            | 5.5(2)                   |
| 0.58(2) | 5.4(2)            | 5.4(2)                   |
| 0.73(1) | 5.2(1)            | 5.2(1)                   |
| 0.85(1) | 5.1(1)            | 5.1(1)                   |
| 0.97(2) | 5.0(2)            | 5.0(2)                   |
| 1       | 4.9(1)            | 4.9(1)                   |

TABLE II. Transition temperature derived from heat capacity (HC,  $H = 0$  T) and AC susceptibility ( $H = 100$  Oe, parallel to  $[110]$ ).

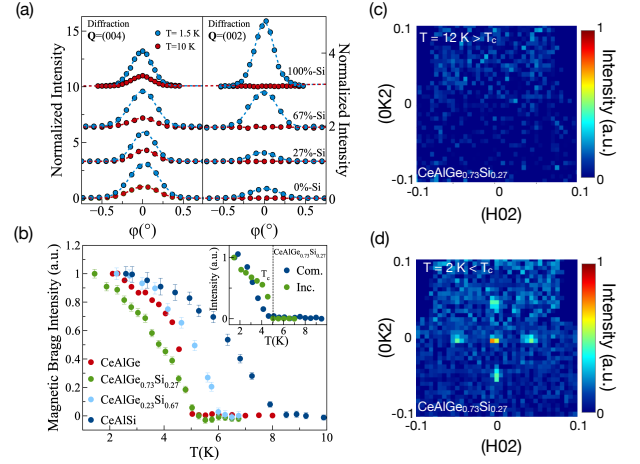

FIG. S5. (a) Rocking scans collected at both  $\mathbf{Q}=(004)$  and  $(002)$  for both  $T=1.5$  K and 10 K using a triple-axis neutron spectrometer. (b) Order parameter measurements collected with neutron diffraction on magnetic Bragg peaks of various doping range  $x$  for  $\text{CeAlSi}_{1-x}\text{Ge}_x$ . Top right inset shows that both commensurate and incommensurate order parameter correlates with the same  $T_c$  for  $\text{CeAlGe}$ . (c) and (d) are respectively the  $T = 12$  K and  $T = 2$  K single-crystal neutron diffraction collected near  $\mathbf{Q}=(002)$  on the  $x=0.73$  sample.

tations for space group  $I4_1md$  with a  $\mathbf{k} = \mathbf{0}$  order: (1)  $\Gamma_2$  with strictly out-of-plane ferromagnetic basis vectors, (2)  $\Gamma_4$  also with out-of-plane basis vectors, but antiferromagnetically coupled between the Ce1 at positions (000) and the Ce2 at positions  $(0,1/2,1/4)$ , and (3)  $\Gamma_5$ , which admits only in-plane spin components.

The observation of magnetic intensity at Bragg positions at  $\mathbf{Q} = (00L)$  implies the presence of in-plane magnetic moments so our data refines best within the  $\Gamma_5$  manifold. Within this manifold, two independent basis vector sets are allowed, enabling independent magnitude and in-plane orientation of the two Ce1 and Ce2 spins forming the primitive unit cell, which we respectively defined as  $\mathbf{S}_1$  and  $\mathbf{S}_2$ .

Intensity at structurally allowed Bragg positions indicates a finite ferromagnetic component  $\mathbf{S}_1 + \mathbf{S}_2 \neq 0$ ,

while intensity at disallowed positions signals a finite antiferromagnetic component  $\mathbf{S}_1 - \mathbf{S}_2 \neq 0$ . This means that both sites are not pointing fully parallel neither fully anti-parallel to each other. We refined both the absolute magnitude of the Ce spin moments and their relative orientation using approximately 30 symmetry nonequivalent Bragg reflections. Refinement gives  $\theta=70(25)^\circ$  with ordered moments of  $1.25(15) \mu_B$  for  $x < x_c$ , while an ordered moments of  $0.7(1) \mu_B$  for  $x > x_c$  was obtained.

The missing spectral weight for  $x > x_c$  is accounted for by the emergence of incommensurate magnetic order, observed only in this doping range. While phase segregation of  $\mathbf{k} = \mathbf{0}$  and  $\mathbf{k}_{inc}$  domains cannot be completely ruled out, the simultaneous onset of both types of order at  $T_C$  (top right inset of Fig. S5(b)) strongly supports their coexistence within the same domains.

Additionally, as discussed in the main text, the incommensurate Bragg intensity remains essentially unchanged through the ferromagnetic domains selection occurring for a  $H_{c1}$  field applied parallel to the  $[010]$  direction. This behavior is inconsistent with a single- $\mathbf{k}_{inc}$  structure and instead supports a  $4\text{-}\mathbf{k}_{inc}$  magnetic order. As shown in Ref. [2] and consistent with our findings, symmetry constraints on this state requires orthogonal spin components between  $\text{Ce}_1$  and  $\text{Ce}_2$  sites. Our refinement for CeAlGe is optimized by the  $\Gamma_2$  manifold, with a general spin structure given by:

$$\mathbf{S}_1 = \begin{pmatrix} \mu_1 \sin(2\pi \mathbf{k}_a \cdot \mathbf{r}) \\ \mu_2 \sin(2\pi \mathbf{k}_b \cdot \mathbf{r}) + m_0 \\ \mu_3 \cos(2\pi \mathbf{k}_a \cdot \mathbf{r}) + \mu_4 \cos(2\pi \mathbf{k}_b \cdot \mathbf{r}) \end{pmatrix} \quad (1)$$

and

$$\mathbf{S}_2 = \begin{pmatrix} \mu_2 \sin(2\pi \mathbf{k}_a \cdot \mathbf{r}) + m_0 \\ \mu_1 \sin(2\pi \mathbf{k}_b \cdot \mathbf{r}) \\ \mu_4 \cos(2\pi \mathbf{k}_a \cdot \mathbf{r}) + \mu_3 \cos(2\pi \mathbf{k}_b \cdot \mathbf{r}) \end{pmatrix} \quad (2)$$

with refined parameters  $\mu_1 = 0.52(8) \mu_B$ ,  $\mu_2 = 0.19(4) \mu_B$ ,  $\mu_3 = 0.35(6) \mu_B$ ,  $\mu_4 = 0.36(6) \mu_B$ , and  $m_0 = 0.7(1) \mu_B$ . The resulting spin structure, illustrated in Fig. S6(a,b), reveals a non-collinear spins arrangement perturbed by a long-wavelength conical spin texture that simultaneously propagates along both the  $\mathbf{a}$  and  $\mathbf{b}$ -axes.

### MONTE CARLO

Our findings can be understood most easily if Weyl electrons are behind the magnetism of  $\text{CeAlSi}_{1-x}\text{Ge}_x$  for  $x > x_c$ . First of all, the DFT identifies Weyl electrons as the only (or main) contributors to the Fermi surface. Then, the interactions between the local moments are mediated by Weyl electrons, given that the band of localized electrons is too narrow to produce a significant superexchange. The complex multi- $\mathbf{k}$  spin structure found via neutron diffraction for  $x > x_c$  also

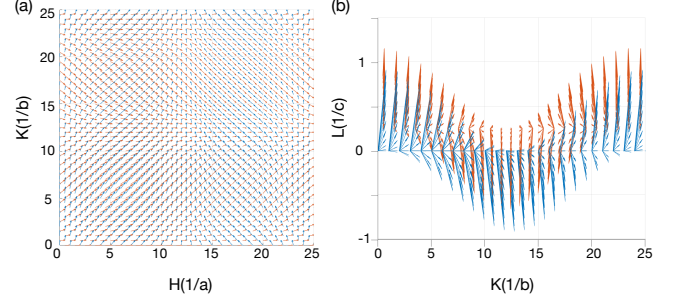

FIG. S6. Spin structure of CeAlGe including both commensurate and incommensurate components. Blue (orange) arrows represent the spins of  $\text{Ce}_1$  ( $\text{Ce}_2$ ) sites. Panel (a) presents the view along the  $c$ -axis (out of the page), while panel (b) shows the view along the  $a$ -axis (out of the page). As illustrated in (b), the spins form a conical arrangement, with  $\text{Ce}_1$  (blue) spins producing a net magnetization along the  $[010]$  direction. In contrast, the  $\text{Ce}_2$  (orange) spins cancel along  $[010]$ . Viewed in the  $(H0L)$  plane, the opposite occurs where the  $\text{Ce}_1$  spins exhibit no net moment, while the  $\text{Ce}_2$  spins contribute a net magnetization along  $[100]$ . Together, these components result in an overall ferromagnetic moment along the  $[110]$  direction.

implies that multiple-spin interactions, beyond the typical Heisenberg and Dzyaloshinskii-Moriya (DM) interactions, play an important role in the “incommensurate” magnetic ordering [3]. Multi-spin interactions are naturally induced by itinerant electrons and hardly intrinsic to well-localized moments. Among them are chiral multi-spin interactions. Theory shows that all chiral interactions induced by Weyl electrons gain strength from the difference between the Fermi energy and the node energy [4], and we note that, according to the DFT, Ge doping grows a set of Weyl hole pockets that could gradually build all chiral spin interactions.

We tested this physical picture using classical Monte Carlo simulations and achieved a good qualitative agreement with the experiment. The relevant spin model is given by the Hamiltonian  $H = H_{\text{CeAlSi}} + H_{\text{chi}}$  on the lattice shown in Fig.1a of the main text. The undoped material CeAlSi is a ferromagnet shaped by easy-axis anisotropy and Heisenberg interactions:

$$H_{\text{CeAlSi}} = -K \sum_{i \in \text{even}} (\mathbf{S}_i \hat{\mathbf{x}})^2 - K \sum_{i \in \text{odd}} (\mathbf{S}_i \hat{\mathbf{y}})^2 - \sum_{ij} J_{ij} \mathbf{S}_i \mathbf{S}_j. \quad (3)$$

The anisotropy  $K$  favors the  $\hat{\mathbf{x}} = \hat{\mathbf{a}}$  or  $\hat{\mathbf{y}} = \hat{\mathbf{b}}$  direction in alternating even/odd  $ab$  layers, as indicated by the DFT; there is no need to include a  $\hat{\mathbf{z}} = \hat{\mathbf{c}}$  direction anisotropy in the minimal model. The ferromagnetic Heisenberg interaction ( $J_{ij} > 0$ ) has extended range in order to capture the influence of itinerant Weyl electrons: the spins are coupled up to three layers apart and up to three lattice constants away in  $ab$  planes. The detailed form of the Heisenberg couplings is the same as in Ref.[5]. The ground state of  $H_{\text{CeAlSi}}$  is the magnetic order found



in CeAlSi, with a 4-fold degeneracy as described in the main text.

Additional interactions are present in the minimal model and grow in strength with Ge doping according to the DFT and field theory [4], eventually leading to a multi- $\mathbf{k}$  magnetic order. A simple Landau-Ginzburg argument paints all 2-spin interactions as unlikely candidates for the explanation of multi- $\mathbf{k}$  orders, and our Monte Carlo calculations confirm that all attempted Heisenberg and Dzyaloshinskii-Moriya couplings stabilize  $2Q$  orders within  $ab$ -planes. At the next level of complexity are 3-spin couplings. Assuming the  $SU(2)$  symmetry, which is appropriate for the interactions induced by isotropic Weyl electrons, only the chiral  $\mathbf{S}_i \cdot (\mathbf{S}_j \times \mathbf{S}_k)$  coupling of spins on three sites  $ijk$  is allowed, but requires an external magnetic field [4]. Therefore, the lowest-level spin interactions that are relevant for the multi- $\mathbf{k}$  order in zero magnetic field are 4-spin couplings. Biquadratic interactions of the form  $(\mathbf{S}_i \cdot \mathbf{S}_j)(\mathbf{S}_k \cdot \mathbf{S}_l)$  have been explored before in two-dimensional models, and can indeed stabilize multi- $\mathbf{k}$  orders that were described as a lattice of “spin vortices” [3]. Alternative 4-spin interactions are chiral,

$$H_{\text{chi}} = \sum_{ijk} \Phi_{ijk} \mathbf{S}_i \cdot (\mathbf{S}_j \times \mathbf{S}_k). \quad (4)$$

This type of interaction emerges naturally in the gauge-theory representation of spin dynamics [4], where ordinary  $U(1)$  gauge fields come from electrodynamics and  $SU(2)$  gauge fields serve as mathematical representations of the microscopic spin-orbit coupling. The full  $U(1) \times SU(2)$  structure of the “flux”  $\Phi_{ijk}$  is

$$\Phi_{ijk} = c_0 B_{ijk} + \varphi_{ijk} \cdot (c_i \mathbf{S}_i + c_j \mathbf{S}_j + c_k \mathbf{S}_k). \quad (5)$$

$B_{ijk}$  is the  $U(1)$  magnetic field component perpendicular to the  $ijk$  plane, providing the 3-spin chiral interaction and acting as a chemical potential for skyrmions. The vector constants  $\varphi_{ijk}$  control the 4-spin  $SU(2)$  part of the chiral interaction, which originates in the spin-orbit coupling. The ideal Weyl spectrum with maximum symmetry cannot introduce any directional bias, and then  $\varphi_{ijk} \perp (ijk)$  couples the  $ijk$  spin chirality

$$\chi_{ijk} = \mathbf{S}_i \cdot (\mathbf{S}_j \times \mathbf{S}_k) \quad (6)$$

only to the spin components that are perpendicular to the  $ijk$  plane. This is the kind of 4-spin chiral interaction that we model here. Other spin projections also become involved when the Weyl spectrum has lower symmetry, e.g. when its dispersion is “tilted”. In principle, the average spin projection on the three sites can be coupled to the chirality, but the geometric inequivalence between the three sites and the specific arrangement of Weyl nodes in the 1st Brillouin zone rarely allow this pristine symmetry to be realized; hence, some generic linear combination of

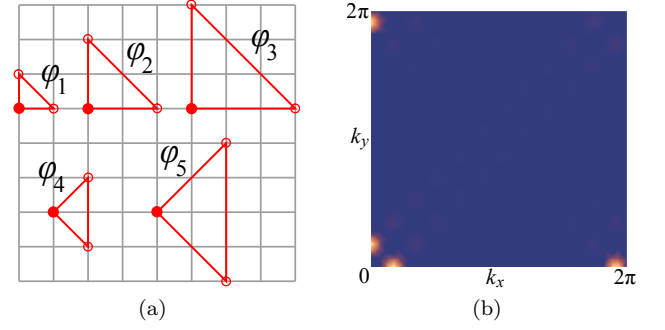

FIG. S7. (a) The site triplets  $ijk$  in the  $ab$ -planes on which the 4-spin chiral interactions are implemented in this study. All symmetry-related triplets are included, and the  $z$  spin projection on the site marked with a solid circle is coupled to the spin chirality on the triangle. (b) The Fourier transform of the  $C(\mathbf{r}) = \sum_{\mathbf{R}} \langle \mathbf{S}(\mathbf{R}) \cdot \mathbf{S}(\mathbf{R} + \mathbf{r}) \rangle$  spin-spin correlation function in an  $ab$ -plane, obtained from the model with typical 4-spin chiral interactions among which  $\phi_5$  is dominant. In this Monte Carlo calculation on the sample with  $2 \times 12^3$  sites,  $\varphi_1 = 1$ ,  $\varphi_2 = 1.5$ ,  $\varphi_3 = 2$ ,  $\varphi_4 = 2.5$ ,  $\varphi_5 = 4$ , with anisotropy  $K = 3$ ,  $ab$ -plane Heisenberg amplitude  $J = 0.55$ , and temperature  $T = 0$ .

spins can be coupled to their chirality, and we model only the simplest realizations of this.

Our choice for this study is to include only a set of chiral interactions within  $ab$ -planes, depicted in Fig.S7(a), and no biquadratic interactions. This is motivated by the anticipated role that Weyl electrons play in inducing the interactions among the local moments. Like the Weyl-induced Heisenberg interactions, the non-chiral biquadratic interactions are expected to be strongest at short distances and spatially modulated at wavevectors derived from the locations of Weyl nodes in the 1st Brillouin zone; this tends to stabilize magnetic orders with large ordering wavevectors  $\mathbf{k}$ , as observed in NdAlSi and SmAlSi [5, 6]. Since the experimentally observed peaks occur at very small wavevectors  $\mathbf{k}$  in CeAlGe, we suspect that chiral interactions are at play: the 2-spin DM interaction can routinely facilitate spiral low- $\mathbf{k}$  orders in ferromagnets, and the 4-spin chiral interactions can naturally achieve analogous low-multi- $\mathbf{k}$  orders.

While exploring the full phase diagram of the above model requires a separate future study, Monte Carlo simulations immediately show that the competition between  $H_{\text{CeAlSi}}$  and  $H_{\text{chi}}$  reproduces the phase transitions that are driven by Ge doping and temperature. Ge doping controls both the amount of easy-axis anisotropy ( $K$ ) and overall strength ( $\varphi_n$ ) of all chiral interactions. Variations of either parameter give rise to 1st order transitions between ferromagnetic and multi- $\mathbf{k}$  magnetic orders at low temperatures. The critical value of the parameter has little or no temperature dependence. The transitions across a critical temperature appear to be of 2nd order in both types of magnetic states. The multi- $\mathbf{k}$  order in the present

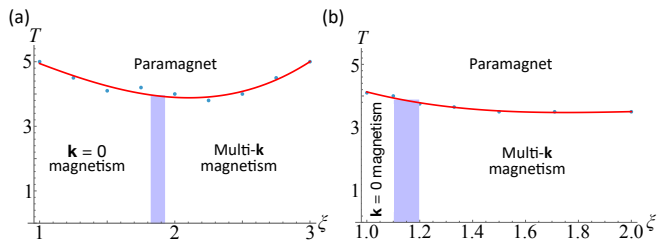

FIG. S8. The doping ( $\xi \sim x$ ) and temperature ( $T$ ) phase diagram calculated with Monte Carlo. (a) Easy-axis anisotropy and chiral interaction strength are both varied with doping; (b) only the anisotropy is varied with doping. The model, units and other details are explained in the text

model is a meron lattice with a diagonal checkerboard of positive and negative chirality tiles, which produces the spin-correlation Fourier transform shown in Fig.S7(b). The experimental set of four peaks at low finite  $\mathbf{Q}$  is reproduced with correct symmetry, while the  $\mathbf{Q} = 0$  intensity is missing. The model ingredients which introduce the  $\mathbf{Q} = 0$  peak without disturbing the other four will be a subject of the future comprehensive study. However, we note two prominent candidate mechanisms. (i) Ferromagnetic Heisenberg interactions induced by Weyl electrons have an extended spatial range, and hence can correlate the in-plane spins at the boundaries between the positive and negative chirality tiles in the meron lattice; the present Monte Carlo has a too short-range of Heisenberg interactions to explore this effect. (ii) The 4-spin chiral couplings should be induced by Weyl electrons on “vertical” lattice triangles in  $ac$  and  $bc$  planes as well. This is not included in the present study, but preliminary Monte Carlo shows that such couplings may also be able to introduce a  $\mathbf{Q} = 0$  peak.

The experimentally obtained phase diagram, shown in the main text in Fig. 1(b), is qualitatively reproduced with the present model. Instead of representing the lattice as combination of Ge and Si sites, doping  $x$  is modeled indirectly by parametrizing via  $\xi$  the doping-dependent easy-axis anisotropy and overall chiral interaction strength in an otherwise homogeneous magnetic lattice. We compare two different parametrizations in Fig.S8: (a)  $K = 3/\xi$ ,  $\xi = \varphi_3$  in which both the easy-axis anisotropy  $K$  and the chiral interaction strength change with doping, and (b)  $K = 3/\xi$ ,  $\varphi_3 = 1$  in which only the anisotropy changes. The former is motivated by the DFT insight into the appearance of additional hole-Weyl-pockets which grow upon GE doping and possibly contribute the chiral interactions, while the latter is motivated by the possibility that the Weyl nodes already present in CeAlSi dominate the chiral interactions in all phases. It turns out that the scenario (b) provides a slightly better qualitative fit of the experiment since it keeps the critical temperature largely independent of doping in the multi- $\mathbf{k}$  phase. All

Heisenberg interactions are kept fixed, with strengths  $J_{c1} = 0.3$ ,  $J_{c2} = 0.2$ ,  $J_{c3} = 0.1$  on the shortest “vertical” links between the 1st, 2nd, 3rd neighbor layers respectively, and amplitude  $J = 0.2$  within the  $ab$  layers (these are of extended range, with the form given in the Supplementary Material of Ref.[5]). The critical temperature is estimated with the following procedure that works both in ferromagnetic and meron (non-coplanar antiferromagnetic) phases. First, a thermally averaged spin vector is registered with Monte Carlo on every lattice site, and then the magnitude of these vectors is averaged over all lattice sites; the temperature dependence of the average spin magnitude exhibits a gradual drop characteristic of a 2nd order transition in the ordered phase, followed by a temperature-independent plateau in the paramagnetic phase (close to zero value, but not zero due to fluctuations; the average magnetization is zero.). The phase diagrams in Fig.S8 depict the temperature  $T$  in the energy units adopted for all couplings in the simulation. The estimates of critical temperature are shown with dots, and fitted with a 3rd order polynomial to guide the eye. The phase transition between ferromagnetic and meron lattice states at critical doping is shown as a vertical blue bar whose thickness represents the resolution of the numerical data.

## DFT

Electronic structure calculations were performed within the framework of density functional theory using the projected augmented wave method as implemented in the Vienna *ab-initio* simulation package (VASP)[7–10]. The generalized gradient approximation (GGA) [11] was employed to account for exchange-correlation effects, and spin-orbit coupling was included self-consistently. The non-magnetic state of CeAlSi and CeAlGe was modeled by treating the Ce  $f$ -electrons as core electrons. We used experimental lattice parameters (CeAlSi:  $a = 4.2520$  Å,  $c = 14.580$  Å, and CeAlGe:  $a = 4.272$  Å,  $c = 14.646$  Å) for all calculations, and the internal atomic positions were relaxed until the residual forces on each atom were less than  $10^{-2}$  eV/Å. A kinetic energy cut-off of 450 eV was employed for the plane-wave basis set. A  $\Gamma$ -centered  $9 \times 9 \times 9$  k-mesh was used for bulk Brillouin zone sampling. The material-specific tight-binding Hamiltonian for CeAlSi and CeAlGe were generated using VASP2WANNIER90 interface [12]. We tabulate the energy, momentum-space positions and chirality of Weyl nodes for CeAlSi and CeAlGe in Table III and IV.

TABLE III. Momentum-space positions, chirality and energies of the Weyl nodes in the non-magnetic state of CeAlSi. A total of 24 Weyl nodes are present, including eight  $W_1$  and sixteen  $W_2$  nodes. The nodes within each set are related by the space group and time-reversal symmetry. The energy is with reference to Fermi level.

| Weyl nodes | $(k_x, k_y, k_z)(\text{\AA}^{-1})$ [Chirality]                                                                                                                                                                                                                                                         | Energy (meV) |
|------------|--------------------------------------------------------------------------------------------------------------------------------------------------------------------------------------------------------------------------------------------------------------------------------------------------------|--------------|
| $W_1$      | $(+0.005, +0.761, 0.000)[+1]$ , $(+0.761, +0.005, 0.000)[-1]$ ,<br>$(-0.005, -0.761, 0.000)[+1]$ , $(-0.761, -0.005, 0.000)[-1]$ ,<br>$(+0.761, -0.005, 0.000)[+1]$ , $(-0.005, +0.761, 0.000)[-1]$ ,<br>$(-0.761, +0.005, 0.000)[+1]$ , $(+0.005, -0.761, 0.000)[-1]$                                 | 108          |
| $W_2$      | $(+0.020, -0.362, \pm 0.259)[+1]$ , $(-0.362, +0.020, \pm 0.259)[-1]$ ,<br>$(-0.020, +0.362, \pm 0.259)[+1]$ , $(+0.362, -0.020, \pm 0.259)[-1]$ ,<br>$(+0.362, +0.020, \pm 0.259)[+1]$ , $(+0.020, +0.362, \pm 0.259)[-1]$ ,<br>$(-0.362, -0.020, \pm 0.259)[+1]$ , $(-0.020, -0.362, \pm 0.259)[-1]$ | 25           |

TABLE IV. Momentum-space positions, chirality and energies of the Weyl nodes in the non-magnetic state of CeAlGe. A total of 40 Weyl nodes are present, including eight  $W_1$ , sixteen  $W_2$ , eight  $W_3^1$  and eight  $W_3^2$  nodes. The nodes within each set are related by the space group and time-reversal symmetry. The energy is with reference to Fermi level.

| Weyl nodes | $(k_x, k_y, k_z)$ [Chirality]                                                                                                                                                                                                                                                                          | Energy (meV) |
|------------|--------------------------------------------------------------------------------------------------------------------------------------------------------------------------------------------------------------------------------------------------------------------------------------------------------|--------------|
| $W_1$      | $(+0.003, -0.748, 0.000)[+1]$ , $(-0.748, +0.003, 0.000)[-1]$ ,<br>$(-0.003, +0.748, 0.000)[+1]$ , $(+0.748, -0.003, 0.000)[-1]$ ,<br>$(-0.748, -0.003, 0.000)[+1]$ , $(-0.003, -0.748, 0.000)[-1]$ ,<br>$(+0.748, +0.003, 0.000)[+1]$ , $(+0.003, +0.748, 0.000)[-1]$                                 | 97           |
| $W_2$      | $(+0.014, +0.373, \pm 0.304)[+1]$ , $(+0.373, +0.014, \pm 0.304)[-1]$ ,<br>$(-0.014, -0.373, \pm 0.304)[+1]$ , $(-0.373, -0.014, \pm 0.304)[-1]$ ,<br>$(-0.373, +0.014, \pm 0.304)[+1]$ , $(+0.014, -0.373, \pm 0.304)[-1]$ ,<br>$(+0.373, -0.014, \pm 0.304)[+1]$ , $(-0.014, +0.373, \pm 0.304)[-1]$ | 59           |
| $W_3^1$    | $(-0.329, +0.265, 0.000)[+1]$ , $(+0.265, -0.329, 0.000)[-1]$ ,<br>$(+0.329, -0.265, 0.000)[+1]$ , $(-0.265, +0.329, 0.000)[-1]$ ,<br>$(+0.265, +0.329, 0.000)[+1]$ , $(+0.329, +0.265, 0.000)[-1]$ ,<br>$(-0.265, -0.329, 0.000)[+1]$ , $(-0.329, -0.265, 0.000)[-1]$                                 | 85           |
| $W_3^2$    | $(-0.360, +0.273, 0.000)[+1]$ , $(+0.273, -0.360, 0.000)[-1]$ ,<br>$(+0.360, -0.273, 0.000)[+1]$ , $(-0.273, +0.360, 0.000)[-1]$ ,<br>$(+0.273, +0.360, 0.000)[+1]$ , $(+0.360, +0.273, 0.000)[-1]$ ,<br>$(-0.273, -0.360, 0.000)[+1]$ , $(-0.360, -0.273, 0.000)[-1]$                                 | 111          |

## REFERENCES

- 
- [1] H.-Y. Yang, B. Singh, J. Gaudet, B. Lu, C.-Y. Huang, W.-C. Chiu, S.-M. Huang, B. Wang, F. Bahrami, B. Xu, *et al.*, [Phys. Rev. B \*\*103\*\*, 115143 \(2021\)](#).
  - [2] P. Puphal, V. Pomjakushin, N. Kanazawa, V. Ukleev, D. J. Gawryluk, J. Ma, M. Naamneh, N. C. Plumb, L. Keller, R. Cubitt, E. Pomjakushina, and J. S. White, [Phys. Rev. Lett. \*\*124\*\*, 017202 \(2020\)](#).
  - [3] R. Ozawa, S. Hayami, K. Barros, G.-W. Chern, Y. Motome, and C. D. Batista, [J. Phys. Soc. Jpn \*\*85\*\*, 103703 \(2016\)](#).
  - [4] P. Nikolić, [Phys. Rev. B \*\*103\*\*, 155151 \(2021\)](#).
  - [5] X. Yao, J. Gaudet, R. Verma, D. E. Graf, H.-Y. Yang, F. Bahrami, R. Zhang, A. A. Aczel, S. Subedi, D. H. Torchinsky, *et al.*, [Phys. Rev. X \*\*13\*\*, 011035 \(2023\)](#).
  - [6] J. Gaudet, H.-Y. Yang, S. Baidya, B. Lu, G. Xu, Y. Zhao, J. A. Rodriguez-Rivera, C. M. Hoffmann, D. E. Graf, D. H. Torchinsky, P. Nikolić, D. Vanderbilt, F. Tafti, and C. L. Broholm, [Nat. Mater. \*\*20\*\*, 1650 \(2021\)](#).
  - [7] P. Hohenberg and W. Kohn, [Phys. Rev. \*\*136\*\*, B864 \(1964\)](#).
  - [8] P. E. Blöchl, [Phys. Rev. B \*\*50\*\*, 17953 \(1994\)](#).
  - [9] G. Kresse and J. Furthmüller, [Physical Review B \*\*54\*\*, 11169 \(1996\)](#).
  - [10] G. Kresse and D. Joubert, [Physical Review B \*\*59\*\*, 1758 \(1999\)](#).
  - [11] J. P. Perdew, K. Burke, and M. Ernzerhof, [Physical Review Letters \*\*77\*\*, 3865 \(1996\)](#).
  - [12] A. A. Mostofi, J. R. Yates, Y.-S. Lee, I. Souza, D. Vanderbilt, and N. Marzari, [Computer Physics Communications \*\*178\*\*, 685 \(2008\)](#).
